# Supplementary material for: Confidence Boosts Trust-Based Resilience in Cooperative Multi-Robot Systems
Source: arXiv:2506.08807 source file (2026-11-26)
Supplement: Supplementary file 1 [file proof-convergence-rate-leg-t-less-tf.tex]

%!TEX root = ../resilient_consensus_trust.tex

\subsection{Convergence Rate of Contribution by Legitimate Robots}

In this part, 
we prove the bound $\rho_\leg(t)$ in~\eqref{eq:convergence-rate-bound-leg-t<tf}.
Considering again the inequality~\eqref{eq:state-mismatch-leg-norm},
we first bound $\norm[\infty]{\Wautleg{t} - \Wautleg{\infty}}$.
Consider the factorization
\begin{equation}\label{eq:leg-weights-prod-fact}
	\Wautleg{t} - \Wautleg{\infty} = \lr I - \prodlamfin{t}{\infty}\prodWleg{k}{t}{\infty}\rr \Wautleg{t}.
\end{equation}
It holds 
\begin{equation}
	\begin{aligned}
		\norm[\infty]{\Wautleg{t}} 
		&= \norm[\infty]{\prodW{k}{0}{t-1}} \\
		&= \prodlamfin{0}{t}\norm[\infty]{\prod_{k=0}^{t-1}W_k^{\mathcal{L}}} \le \prodlamfin{0}{t}\cdot 1=\prodlamfin{0}{t}.
\end{aligned}
\end{equation}
This is the tightest possible bound for $\Wautleg{t}$ because legitimate robots might distrust all neighbors before time $\tf$ in the worst case that requires upper bounding $\norm[\infty]{\prod_{k=0}^{t-1}W_k^{\mathcal{L}}}\le 1$.
As for the first factor,
it holds
\begin{equation}
		\prodWleg{k}{t}{\infty}	= \lr\Wlegtrue\rr^\infty \prodWleg{k}{t}{\tf-1} 
									= \one v^{\top} \prodWleg{k}{t}{\tf-1}
\end{equation}
and we can lower bound the diagonal elements as
\begin{equation}\label{eq:leg-weights-diag-bound}
	\begin{aligned}
		\ls\one v^{\top}\prodWleg{k}{t}{\tf-1}\rs_{ii}	&\ge \vmin \ls\prodWleg{k}{t}{\tf-1}\rs_{ii}
															\ge \vmin \prod_{k=t}^{\tf}\ls\Wleg{k}\rs_{ii}\\
															&\ge \dfrac{\vmin}{(\dmax+1)^{\tf-t+1}}.
	\end{aligned}
\end{equation}
Combining~\eqref{eq:leg-weights-diag-bound} with \cref{lem:matrix-difference} yields
\begin{equation}
	\norm[\infty]{I - \prodlamfin{t}{\infty}\prodWleg{k}{t}{\infty}} \le 
	2\lr1 - \dfrac{\prodlamfin{t}{\infty}\vmin}{(\dmax+1)^{\tf-t+1}}\rr
\end{equation}
and from~\eqref{eq:leg-weights-prod-fact} it follows
\begin{equation}\label{eq:leg-weights-prod-norm-bound}
	\norm[\infty]{\Wautleg{t} - \Wautleg{\infty}} \le 2\prodlamfin{0}{t-1}\lr 1 - \dfrac{\prodlamfin{t}{\infty}\vmin}{(\dmax+1)^{\tf-t+1}}\rr.
\end{equation}
We now bound $\norm[\infty]{\Winleg{t} - \Winleg{\infty}}$.
Rewrite $\Winleg{t} - \Winleg{\infty}$ as
\begin{multline}\label{eq:B_t-B-inf-decomp}
	\Winleg{t} - \Winleg{\infty} = \sum_{k=0}^{t-2}\prodlamfin{k+1}{t-1}C_k^{t-1}\lam{k} + \lam{t-1}I \\
	+ \sum_{k=t}^{\infty} \lr\prodW{s}{k+1}{t-1}\rr\lam{k}
\end{multline}
with $C_k^{t-1}$ defined in~\eqref{eq:C}.
The induced norm of the first summation in~\eqref{eq:B_t-B-inf-decomp} can be upper bounded using the triangle inequality.
For each element in this summation,
the same argument used to bound $\norm[\infty]{\Wautleg{t} - \Wautleg{\infty}}$ applies with the difference that the products start from $k+1$.
It follows that
\begin{equation}\label{eq:bound-C}
	\norm[\infty]{C_k^{t-1}} \le 2\prodlamfin{k+1}{t-1}\lr 1 - \dfrac{\prodlamfin{t+1}{\infty}\vmin}{(\dmax+1)^{\tf-t+1}}\rr.
\end{equation}
Since all matrices $\Wleg{t}$ are sub-stochastic,
it holds
\begin{equation}\label{eq:B_t-second-summation-tf}
	\norm[\infty]{\lr\prodW{s}{k+1}{t-1}\rr\lam{k}} \le \prodlamfin{k+1}{\infty}\lam{k}.
\end{equation}
Combining~\eqref{eq:B_t-B-inf-decomp} with~\eqref{eq:bound-C} and~\eqref{eq:B_t-second-summation-tf} via the triangle inequality yields
\begin{multline}\label{eq:leg-weights-sum-norm-bound}
	\norm[\infty]{\Winleg{t} - \Winleg{\infty}} \le \sum_{k=0}^{t-2}2\prodlamfin{k+1}{t-1}\lr 1 - \dfrac{\prodlamfin{t}{\infty}\vmin}{(\dmax+1)^{\tf-t+1}}\rr\lam{k} \\
	+ \lam{t-1} + \sum_{k=t}^{\infty}\prodlamfin{k+1}{\infty}\lam{k}.
\end{multline}
Combining~\eqref{eq:state-mismatch-leg-norm} with~\eqref{eq:leg-weights-prod-norm-bound} and~\eqref{eq:leg-weights-sum-norm-bound} yields $\rho_\leg(t)$ in~\eqref{eq:convergence-rate-bound-leg-t<tf}.
