# Supplementary material for: Confidence Boosts Trust-Based Resilience in Cooperative Multi-Robot Systems
Source: arXiv:2506.08807 source file (2026-11-26)
Supplement: Supplementary file 2 [file proof-convergence-rate-mal-t-less-tf.tex]

%!TEX root = ../resilient_consensus_trust.tex

\subsection{Convergence Rate of Contribution by Malicious Robots}

We next prove the bound $\rho_\mal(t)$ in~\eqref{eq:convergence-rate-bound-mal-t<tf}.
It holds
\begin{multline}
	\statecontrmal{t} - \statecontrmalss = 
	\sum_{k=0}^{t-1} C_k^{t-1} (1-\lam{k})\Wmal{k}\statemal{k} \\
	+ \sum_{k=t}^{\tfmal-1}\lr\prodlamfin{k+1}{\infty}\prodWleg{s}{k+1}{\infty}\rr (1-\lam{k})\Wmal{k}\statemal{k}.
\end{multline}
For $t\le\tfmal\le\tf$,
the triangle inequality combined with~\eqref{eq:bound-C} and~\eqref{eq:contr-mal-bound},
bounds the first summation in~\eqref{eq:state-mismatch-mal-1} as
\begin{multline}\label{eq:contr-mal-prod-bound}
	\norm[\infty]{\sum_{k=0}^{t-1} C_k^{t-1} (1-\lam{k})\Wmal{k}\statemal{k}} \le \\
	\sum_{k=0}^{t-1} 2D_1\eta\prodlamfin{k+1}{t-1}\lr 1 - \dfrac{\prodlamfin{t}{\infty}\vmin}{(\dmax+1)^{\tf-t+1}}\rr(1-\lam{k}).
\end{multline}
Using~\eqref{eq:contr-mal-bound},
for the second summation in~\eqref{eq:state-mismatch-mal-1} it holds
\begin{multline}\label{eq:contr-mal-sum-bound}
	\norm[\infty]{\sum_{k=t}^{\tfmal-1}\lr\prodlamfin{k+1}{\infty}\prodWleg{s}{k+1}{\infty}\rr (1-\lam{k})\Wmal{k}\statemal{k}} \le \\
	\sum_{k=t}^{\tfmal-1} D_1\eta\prodlamfin{k+1}{\infty}(1-\lam{k}).
\end{multline}
Finally,
combining~\eqref{eq:state-mismatch-mal-1} with~\eqref{eq:contr-mal-bound} and~\eqref{eq:contr-mal-prod-bound}--\eqref{eq:contr-mal-sum-bound} through the triangle inequality,
the quantity $\norm[\infty]{\statecontrmal{t}-\statecontrmalss}$ is bounded by $\rho_\mal(t)$ in~\eqref{eq:convergence-rate-bound-mal-t<tf}.
