# Supplementary material for: Confidence Boosts Trust-Based Resilience in Cooperative Multi-Robot Systems
Source: arXiv:2506.08807 source file (2026-11-26)
Supplement: Supplementary file 3 [file proof-convergence-rate-t-less-tf.tex]

%!TEX root = ../resilient_consensus_trust.tex

\section{Proof of \cref{prop:convergence-rate-before-tf}}
\label{ass:proof-convergence-rate-t-less-tf}

We start again from the inequality~\eqref{eq:convergence-error}.
