# Supplementary material for: Confidence Boosts Trust-Based Resilience in Cooperative Multi-Robot Systems
Source: arXiv:2506.08807 source file (2026-11-26)
Supplement: Supplementary file 5 [file final-time-misclassification.tex]

%!TEX ROOT = ../resilient_consensus_trust.tex

\section{Probability of Correct Classification Time}
\label{app:final-time-misclassification}

In this appendix,
we compute bounds for the probability of the events $\tfmal=k$ and $\tf=k$,
for some $k\ge0$.
