# Supplementary material for: Confidence Boosts Trust-Based Resilience in Cooperative Multi-Robot Systems
Source: arXiv:2506.08807 source file (2026-11-26)
Supplement: Supplementary file 6 [file proof-convergence-rate-leg-doubly-stochastic.tex]

%!TEX root = ../resilient_consensus_trust.tex

\subsection{Convergence Rate of Contribution by Legitimate Robots}
\label{ass:proof-convergence-rate-leg}

In this part,
we prove the bound $\rho_\leg(t)$ in~\eqref{eq:convergence-rate-bound-leg-t>tf}.
By definition,
the mismatch between the state contribution at time $t$ and the final (asymptotic) value is
\begin{equation}\label{eq:state-mismatch-leg}
	\begin{aligned}
		\statecontrleg{t} - \statecontrlegss	&= (\Wautleg{t} + \Winleg{t})\stateleg{0} - (\Wautleg{\infty} + \Winleg{\infty})\stateleg{0}\\
												&= (\Wautleg{t} - \Wautleg{\infty} + \Winleg{t} - \Winleg{\infty}) \stateleg{0}
	\end{aligned}
\end{equation}
where
\begin{gather}
	\Wautleg{\infty} \doteq \lim_{t\rightarrow\infty}\Wautleg{t}
	\qquad \Winleg{\infty} \doteq \lim_{t\rightarrow\infty}\Winleg{t}.
\end{gather}
From~\eqref{eq:state-mismatch-leg},
it follows
\begin{multline}\label{eq:state-mismatch-leg-norm}
		\norm[\infty]{\statecontrleg{t} - \statecontrlegss}	\le \norm[\infty]{\Wautleg{t} - \Wautleg{\infty}}\norm[\infty]{\stateleg{0}} \\
		+ \norm[\infty]{\Winleg{t} - \Winleg{\infty}}\norm[\infty]{\stateleg{0}}.
\end{multline}
We next upper bound the two induced matrix norms in~\eqref{eq:state-mismatch-leg-norm}.
We first bound $\norm[\infty]{\Wautleg{t} - \Wautleg{\infty}}$.
We factor out the first $\tf$ matrix factors of $\Wautleg{t} - \Wautleg{\infty}$ and the common factor $\prodlamfin{\tf}{t-1}$:
\begin{equation}\label{eq:leg-weights-prod-fact-t>tf}
	\begin{aligned}
		\Wautleg{t} - \Wautleg{\infty}	&= \lr \prodWleg{k}{\tf}{t-1} - \prodlamfin{t}{\infty}\prodWleg{k}{\tf}{\infty}\rr \prodlamfin{\tf}{t-1} \Wautleg{\tf-1}\\
		&= \lr \lr\Wlegtrue\rr^{t-\tf} - \prodlamfin{t}{\infty}\lr\Wlegtrue\rr^{\infty}\rr \prodlamfin{\tf}{t-1} \Wautleg{\tf-1}.
	\end{aligned}
\end{equation}
We now use the triangle inequality and separately bound the induced matrix norms of the two factors in~\eqref{eq:leg-weights-prod-fact-t>tf}.
The second factor can be bounded as $\norm[\infty]{\prodlamfin{\tf}{t-1} \Wautleg{\tf-1}}\le\prodlamfin{0}{t-1}$.
For generic $\tau$,
we bound the first factor as follows,
\begin{multline}\label{eq:w-true-diff-triangle}
	\norm[\infty]{\lr\Wlegtrue\rr^{\tau} - \prodlamfin{t}{\infty}\lr\Wlegtrue\rr^{\infty}} \le 
	\norm[\infty]{\lr\Wlegtrue\rr^{\tau} - \lr\Wlegtrue\rr^{\infty}} \\
	+ \norm[\infty]{\lr\Wlegtrue\rr^{\infty} - \prodlamfin{t}{\infty}\lr\Wlegtrue\rr^{\infty}}.
\end{multline}
Recall that $\{\sigma_i\}_{i=1}^L$ denotes the singular values of the nominal weight matrix $\Wlegtrue$ sorted in decreasing order.
For the first addend in~\eqref{eq:w-true-diff-triangle},
we use the singular value decomposition $\Wlegtrue=U\Sigma V^\top$,
where we respectively denote the $i$th columns of $U$ and $V$ by $u_i$ and $v_i$,
and with singular values $\sigma_i\doteq\Sigma_{ii}$ sorted in decreasing order such that $\sigma_1 = 1$,
$u_1 = \one$,
and $v_1 = v$:
\begin{equation}
	\lr\Wlegtrue\rr^{\tau} - \lr\Wlegtrue\rr^{\infty}	= \sum_{i=1}^{L}\sigma_i^\tau u_iv_i^\top - \one v^\top
	= \sum_{i=2}^{L}\sigma_i^\tau u_iv_i^\top.
\end{equation}
Because $u_i$ and $v_i$ are stochastic vectors for every $i$,
it follows
\begin{equation}\label{eq:bound-leg-sigma}
	\norm[\infty]{\lr\Wlegtrue\rr^{t-\tf} - \lr\Wlegtrue\rr^{\infty}} \le \sum_{i=2}^{L}\sigma_i^{t-\tf}.
\end{equation}
For the second addend in~\eqref{eq:w-true-diff-triangle},
we readily have
\begin{equation}\label{eq:bound-leg-inf}
	\begin{aligned}
		\norm[\infty]{\lr\Wlegtrue\rr^{\infty} - \prodlamfin{t}{\infty}\lr\Wlegtrue\rr^{\infty}} &= \lr1-\prodlamfin{t}{\infty}\rr\norm[\infty]{\lr\Wlegtrue\rr^{\infty}}\\
		&= 1-\prodlamfin{t}{\infty}.
	\end{aligned}
\end{equation}
Combining~\eqref{eq:leg-weights-prod-fact-t>tf} with~\eqref{eq:w-true-diff-triangle}--\eqref{eq:bound-leg-inf} yields
\begin{equation}\label{eq:leg-weights-prod-norm-bound-t>tf}
	\norm[\infty]{\Wautleg{t}-\Wautleg{\infty}} \le \prodlamfin{0}{t-1}\lr \sum_{i=2}^{L}\sigma_i^{t-\tf} +  1-\prodlamfin{t}{\infty} \rr.
\end{equation}
We now bound $\norm[\infty]{\Winleg{t} - \Winleg{\infty}}$.
We first set apart the last term in the summation within $\Winleg{t}$:
\begin{equation}\label{eq:B_t-split-tf}
	\Winleg{t} = \sum_{k=0}^{t-2} \lr\prodlamfin{k+1}{t-1}\prodWleg{s}{k+1}{t-1}\rr\lam{k} + \lam{t-1}I.
\end{equation}
In this way,
the product within each term of the summation in~\eqref{eq:B_t-split-tf} is never empty.
The same holds for $\Winleg{\infty}$ with the limit $\lam{\infty} = 0$.
Defining
\begin{equation}
	C_k^t \doteq \prodlamfin{k+1}{t}\prodWleg{s}{k+1}{t} - \prodlamfin{k+1}{\infty}\prodWleg{s}{k+1}{\infty},
\end{equation}
we rewrite $\Winleg{t} - \Winleg{\infty}$ as
\begin{multline}\label{eq:B_t-B-inf-decomp-tf}
	\Winleg{t} - \Winleg{\infty}	\nonumber\\
    = \sum_{k=0}^{t-2}C_k^{t-1}\lam{k}  - \sum_{k=t}^{\infty}\lr\prodlamfin{k+1}{\infty}\prodWleg{s}{k+1}{\infty}\rr\lam{k}
	+ \lam{t-1}.
\end{multline}
We factor $C_k^t$ analogously to~\eqref{eq:leg-weights-prod-fact-t>tf} as
\begin{multline}
	C_k^{t-1} = \lr \lr\Wlegtrue\rr^{t-(\maxof{\tf}{(k+1)})} - \prodlamfin{t}{\infty}\lr\Wlegtrue\rr^{\infty}\rr \\
	\cdot \prodlamfin{k+1}{t-1} \prodWleg{s}{k+1}{(\maxof{\tf}{(k+1)})-1}
\end{multline}
and,
in analogy to~\eqref{eq:w-true-diff-triangle}--\eqref{eq:bound-leg-inf},
we obtain
\begin{equation}\label{eq:bound-C-t>tf}
	\norm[\infty]{C_k^{t-1}} \le \prodlamfin{k+1}{t-1}
	\lr \sum_{i=2}^{L}\sigma_i^{t-(\maxof{\tf}{(k+1)})} +  1-\prodlamfin{t}{\infty} \rr.
\end{equation}
As for the second summation in~\eqref{eq:B_t-B-inf-decomp-tf},  the triangle inequality yields
\begin{equation}\label{eq:B_t-second-summation-tf}
	\norm[\infty]{\sum_{k=t}^{\infty}\lr\prodlamfin{k+1}{\infty}\prodWleg{s}{k+1}{\infty}\rr\lam{k}} \le \sum_{k=t}^{\infty}\prodlamfin{k+1}{\infty}\lam{k}.
\end{equation}
Combining~\eqref{eq:B_t-B-inf-decomp-tf} with~\eqref{eq:bound-C-t>tf} and~\eqref{eq:B_t-second-summation-tf} yields
\begin{multline}\label{eq:leg-weights-sum-norm-bound-t>tf}
	\norm[\infty]{\Winleg{t} - \Winleg{\infty}} \le \sum_{k=0}^{t-2}\prodlamfin{k+1}{t-1}\lam{k}\bar{\rho}(t,\maxof{\tf}{(k+1)}) \\
	+ \lam{t-1} + \sum_{k=t}^{\infty}\prodlamfin{k+1}{\infty}\lam{k}
\end{multline}
where $\bar{\rho}$ is defined in~\eqref{eq:convergence-rate-bound-dynamics-t>tf}.
Combining~\eqref{eq:state-mismatch-leg-norm} with~\eqref{eq:leg-weights-prod-norm-bound-t>tf} and~\eqref{eq:leg-weights-sum-norm-bound-t>tf},
we get $\rho_\leg(t)$ in~\eqref{eq:convergence-rate-bound-leg-t>tf}.
