# Supplementary material for: Confidence Boosts Trust-Based Resilience in Cooperative Multi-Robot Systems
Source: arXiv:2506.08807 source file (2026-11-26)
Supplement: Supplementary file 7 [file substochastic-input-matrix.tex]

%!TEX ROOT = ../resilient_consensus_trust.tex

\section{Proof of \cref{lem:prod-w-substochastic}}
\label{app:substochastic-sequence}

The claim follows trivially if $t_1> t_2$ because
the summation is empty.
For $t_1\le t_2$,
we prove~\eqref{eq:prod-lam-less-1} by induction on $t_2$.
\begin{description}
	\item[Base step:] Let $t_2= t_1$,
	then
	\begin{equation}\label{eq:induction-base}
		\sum_{t=t_1}^{t_1}\lr\prodlam{s}{t+1}{t_1} \rr\lam{t} = \lam{t_1} \le1.
	\end{equation}
	\item[Induction step:] Let $t_2>t_1$ and assume that
	\begin{equation}\label{eq:sum-t2}
		\sum_{t=t_1}^{t_2}\lr\prodlam{s}{t+1}{t_2} \rr\lam{t} \le1.
	\end{equation}
	For $t_2+1$,
	it holds
	\begin{multline}\label{eq:convex-comb-lam}
		\sum_{t=t_1}^{t_2+1}\lr\prodlam{s}{t+1}{t_2+1} \rr\lam{t} = \lam{t_2+1} + \\ (1-\lam{t_2+1})\sum_{t=t_1}^{t_2}\lr\prodlam{s}{t+1}{t_2} \rr\lam{t}.
	\end{multline}
	The right-hand side of~\eqref{eq:convex-comb-lam} is a convex combination between $1$ and the left-hand side of~\eqref{eq:sum-t2} with respective coefficients $\lam{t_2+1}$ and $1-\lam{t_2+1}$.
	Therefore,
	noting that all terms are nonnegative,
	by virtue of~\eqref{eq:sum-t2} the left-hand side of~\eqref{eq:convex-comb-lam} is at most $1$,
	completing the proof of~\eqref{eq:prod-lam-less-1}.
\end{description}
The fact that the upper bound is sharp if $\lam{t}\equiv1$ follows by replacing $\lam{t}\equiv1$ in~\eqref{eq:induction-base}--\eqref{eq:sum-t2}.
For the second claim,
it holds
\begin{multline}\label{eq:prod-W}
	\norm[\infty]{\sum_{t=t_1}^{t_2}\lr\prodW{s}{t+1}{t_2} \rr\lam{t}} \\
	\begin{aligned}
		&\stackrel{(i)}{\le}\sum_{t=t_1}^{t_2}\norm[\infty]{\lr\prodW{s}{t+1}{t_2} \rr\lam{t}}\\
		&=\sum_{t=t_1}^{t_2}\lr\prodlam{s}{t+1}{t_2}\rr\norm[\infty]{\prodWleg{s}{t+1}{t_2} }\lam{t}\\
		&\stackrel{(ii)}{\le}\sum_{t=t_1}^{t_2}\lr\prodlam{s}{t+1}{t_2}\rr\lam{t}
	\end{aligned}
\end{multline}
where $(i)$ is the triangle inequality and $(ii)$ follows because the product of sub-stochastic matrices is sub-stochastic.
Claim~\eqref{eq:prod-W-substochastic} follows by combining~\eqref{eq:prod-W} with~\eqref{eq:prod-lam-less-1} and from the definition of induced-infinity norm of matrices by further noting that the matrix in the left-hand side of~\eqref{eq:prod-W} is positive.
If $\lam{t}\equiv1$,
all products inside the summation are empty and the sum reduces to the term $\lam{t_2}I= I$.
